# Supplementary material for: Controlling the shape of membrane protein polyhedra
Source: arXiv:1704.06225 source file (2017-04-20)
Supplement: Supplementary file 1 [file sm.pdf]

# Controlling the shape of membrane protein polyhedra
## Supplementary Material

Di Li, Osman Kahraman, and Christoph A. Haselwandter

*Department of Physics & Astronomy and Molecular and Computational Biology Program, Department of Biological Sciences, University of Southern California, Los Angeles, CA 90089, USA*

### MPPN SELF-ASSEMBLY DIAGRAM FOR VARYING $K_b$ AND $K_t$

To calculate the MPPN self-assembly diagram in fig. 4 of the main text we assume [1, 2], for simplicity, that $K_b$ and $K_t$ are constant with $m$. However, in general $K_b$ and $K_t$ are expected [3] to vary with $m$. To check the robustness of our model predictions with respect to variations in $K_b$ and $K_t$ with $m$, we re-calculated the MPPN self-assembly diagram in fig. 4 of the main text allowing for variations in $K_b$ and $K_t$ over the range of values suggested by experiments [3]. In particular, we proceeded similarly as in refs. [1, 2] and interpolated between experimental data points for the saturated lipids in ref. [3], as follows:

$$K_b = (-25.0645 + 11.2903 \times 2m)\, k_B T\,, \tag{S1}$$

$$K_t = (59.3323 - 0.6452 \times 2m)\, k_B T/\mathrm{nm}^2\,, \tag{S2}$$

where, as in the main text, $2m$ denotes the hydrophobic thickness of the unperturbed lipid bilayer, measured in units of nm. Figure S1(a) shows the MPPN self-assembly diagram obtained using constant $K_b$ and $K_t$ as in fig. 4 of the main text, while fig. S1(b) shows the corresponding MPPN self-assembly diagram obtained using eqs. (S1) and (S2). Allowing for varying $K_b$ and $K_t$ we find that, compared to fig. 4 of the main text, the boundaries of regions of parameter space dominated by distinct $n$-states of MPPNs are shifted. However, the key model predictions described in the main text remain unchanged. In particular, increasing $|U|$ biases the MPPN self-assembly diagram towards highly symmetric and uniform MPPN shapes with $n = 12$, 24, and 48. Thus, our key model predictions are robust with respect to variations in $K_b$ and $K_t$ with $m$.

[1] P. Wiggins and R. Phillips, Proc. Natl. Acad. Sci. U.S.A. **101**, 4071 (2004).

[2] P. Wiggins and R. Phillips, Biophys. J. **88**, 880 (2005).

[3] W. Rawicz, K. Olbrich, T. McIntosh, D. Needham, and E. Evans, Biophys. J. **79**, 328 (2000).

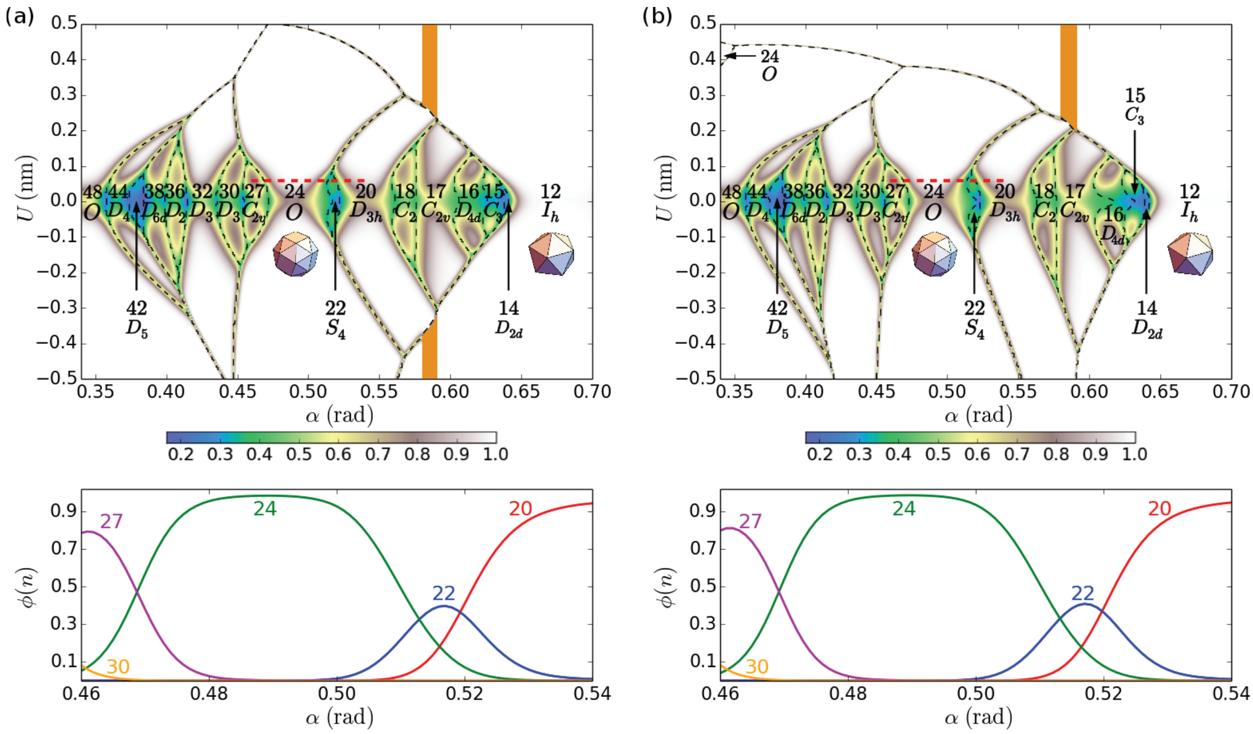


FIG. S1: MPPN self-assembly diagram as a function of bilayer-protein hydrophobic thickness mismatch $U$, which we change by varying $m$, and bilayer-protein contact angle $\alpha$, calculated (a) using $K_b = 14\ k_BT$ and $K_t = 56.5\ k_BT/\text{nm}^2$ as in fig. 4 of the main text and (b) using eqs. (S1) and (S2).
